# Supplementary material for: FAR: Flexible, Accurate and Robust 6DoF Relative Camera Pose Estimation
Source: arXiv:2403.03221 source file (2024-03-05)
Supplement: Supplementary file 1 [file ablations.tex]

\begin{table}[h]
\vspace{-0.5em}

\resizebox{\ifdim\width>\columnwidth \columnwidth \else \width \fi}{!}{
\begin{tabular}{l c c c c c c} \toprule
  & \multicolumn{3}{c}{Translation (m)} & \multicolumn{3}{c}{Rotation ($^{\circ}$)} \\
\textit{Transformer: 8-Point ViT} & Med.$\downarrow$ & Avg.$\downarrow$ & $\leq$1m$\uparrow$ & Med.$\downarrow$ & Avg.$\downarrow$ & $\leq$30$\uparrow$ \\
\midrule
LoFTR + Solver + Scale $\TB_s$ & 0.85 & 1.21 & 56.3 & \textbf{0.26} & 9.66 & 91.2 \\
LoFTR + Updated Solver + Scale $~\TB_u$ & \textbf{0.83} & \textbf{1.17} & \textbf{57.5} & \textbf{0.26} & \textbf{6.62} & \textbf{93.7} \\
\\
\textit{Transformer: Vanilla TF}\\
\midrule
LoFTR + Solver + Scale $\TB_s$ & 0.85 & 1.21 & 56.3 & \textbf{0.26} & 9.66 & 91.2 \\
LoFTR + Updated Solver + Scale $~\TB_u$ & \textbf{0.83} & \textbf{1.17} & \textbf{57.2} & \textbf{0.26} & \textbf{7.30} & \textbf{93.2} \\
\bottomrule 
\end{tabular}
}
\vspace{-1.3em}
\end{table}
